# Supplementary material for: FlexDrive: Toward Trajectory Flexibility in Driving Scene Reconstruction and Rendering
Source: arXiv:2502.21093 source file (2025-03-03)
Supplement: Supplementary file 1 [file X_suppl.tex]

% \clearpage
% \setcounter{page}{0}
% \maketitlesupplementary
\section{FID Score is not a Reliable Criteria for Image Synthesis}\label{FID}
The Fréchet inception distance (FID) is a metric for measuring the distance between two distributions. With the normal distribution assumption, FID scores can be computed with the following formula:
\begin{equation}
    FID = \|\mu_1-\mu_2\|+\rm{Tr}(\sigma_1+\sigma_2-2\sqrt{\sigma_1*\sigma_2})
\end{equation}
In our setting, we compute the FID scores between the in-vehicle path views $(\mu_1,\sigma_1)$ and the rendered shifted views $(\mu_2,\sigma_2)$. Because the shifted views are different from the in-vehicle path views by nature, thus $\mu_1\neq\mu_2$ and $\sigma_1\neq\sigma_2$. Now even if we simply shift the mean of $\mu_2$ to $\mu_1$, we can reduce the FID scores lower than the GT views. For this reason, we claim that FID score is not a good metric for the flexible rendering task.

\section{Effect of Depth Bootstrap}
\label{sec:impl}
\section{Alpha Blended Depth}
In our approach, depth prediction is crucial. To facilitate the original 3D Gaussian splatting field with our depth prediction, we render depth views in a normalized alpha-blending manner, which follows
\begin{equation}
    \label{total_depth}
    D = \frac{1}{\sum_{i=1}^{N}T_i\alpha_i}\sum_{i=1}^{N}{\alpha}_i T_id_i\; {\rm{with}}\; T_i = \prod_{j=1}^{i-1}(1-{\alpha}_j),
\end{equation}
Here $d_i$ is the depth of the 3D Gaussian center with respect to the current camera location. The blended depth can be directly viewed as a weighted average of Gaussian points' depth based on their importance.
\section{Dynamic color encoding}
In a highly dynamic environment, the color of the same object usually changes slightly at different locations or times. To compensate for this phenomenon, we adopted a Dynamic color encoding mechanism similar to 4D Gaussian~\cite{wu20244d}, PVG~\cite{chen2023periodic}, and StreetGaussian~\cite{yan2024street}. We approximate the color-changing with a Taylor series. 

\subsection{Dynamic Objects}
Let $(x_{o},y_{o},z_{o})$ be the logistic coordinates of a Gaussian primitive, and $(l,w,h)$ be the length, width, and height of the bounding box containing this Gaussian primitive. We convert the logistic coordinates into Euclidean coordinates as following 
\begin{align}
        \begin{bmatrix}
{x}_{t}\\
{y}_{t}\\
{z}_{t}\\
\end{bmatrix} = 
\begin{bmatrix}
l(\sigma(x_{o})-0.5)\\
w(\sigma(y_{o})-0.5)\\
h(\sigma(z_{o})-0.5)\\
\end{bmatrix}.
\end{align}
Next, we transform these local Euclidean coordinates into the world coordinates system. As widely used in the community, We introduce a sequence of \textit{trainable} pose parameters $R_t$ and $T_t$. Here $R_t$ is a rotation matrix to transform the local system to the world system at time frame $t$, $T_t$ is the respective offset vector. Then, the world coordinates $(\bar{x}_t,\bar{y}_t,\bar{z}_t)$ can be computed as:
\begin{align}
        \begin{bmatrix}
\bar{x}_{t}\\
\bar{y}_{t}\\
\bar{z}_{t}\\
\end{bmatrix} = 
R_t\begin{bmatrix}
x_{t}\\
y_{t}\\
z_{t}\\
\end{bmatrix}+T_t.
\end{align}

\section{Detailed Training Settings}
In our experiments, we employed the Adam optimizer with a base learning rate of $2.5e-3$.  We focused on two primary hyperparameters relevant to our methods: the bootstrap update interval and the occlusion-aware Inverse View Warping. For the depth bootstrap strategy, we updated the accumulated sparse LiDAR map every $2$ epoch, integrating $30$ frames of LiDAR data into a single sparse depth map. 
In the Inverse View Warping module, we adopt $\beta = 0.95$.
